# Supplementary material for: Structure-Informed Protein Language Model
Source: arXiv:2402.05856 source file (2024-02-07)
Supplement: Supplementary file 1 [file 05_appendix.tex]

\section{More Related Work and Broader Impact}
\label{app:sec:related}

\textbf{Protein Retriever.}
In the domain of proteins, retriever-based methods have long been employed for function annotation~\citep{conesa2005blast2go}, utilizing both sequence~\citep{altschul1990basic,melvin2011detecting,buchfink2021sensitive,Hamamsy2023ProteinRH} and structure-based approaches~\citep{Shindyalov1998ProteinSA,Yang2006ProteinSD,Zhao2013SSWLA,Holm2019BenchmarkingFD,trinquier2022swampnn,greener2022fast,van2023fast}.
Recent endeavors have extended retrievers to retrieve similar sequences from expansive databases, augmenting inputs and subsequently enhancing function prediction performance~\citep{ma2023retrieved,zou2023antibody,dickson2023fine,kilinc2023improved,chen2023learning}. 
Instead of designing a new protein retriever, our work proposes a general strategy to train a neural structure retriever and studies how to use the idea of inter-protein similarity modeling to improve function annotation accruacy.
% In comparison, our work is the first to comprehensively benchmark both sequence- and structure-based retrievers alongside predictors for function annotation tasks.

\textbf{Protein Network Propagation for Function Prediction.}
Besides directly measuring inter-protein similarities based on sequences and structures, there is a parallel line of research that focuses on function annotation through protein-protein interaction (PPI) networks, exemplified by tools like STRING~\citep{szklarczyk2019string}. These networks map both direct physical and indirect functional interactions among proteins.
Recent approaches in this domain involve functional label propagation within these networks~\citep{mostafavi2008genemania,wang2017prosnet,you2019netgo,cho2016compact,kulmanov2018deepgo,yao2021netgo}, and adapting these methods to PPI networks of newly sequenced species~\citep{you2021deepgraphgo,torres2021protein}. However, a key limitation of these methods is that they are not able to make predictions for newly sequenced proteins absent in existing PPI networks.
Moreover, knowing protein-protein interactions is essentially a more difficult challenge, as it requires a more comprehensive understanding of protein properties. 
These problems make this line of work hard to use in real-world settings.

\section{Dataset Details}
\label{app:exp:dataset}

\begin{table}[!h]
    \centering
    \caption{Dataset statistics.}
    \label{tab:dataset}
    \begin{adjustbox}{max width=0.7\linewidth}
        %\footnotesize
        \begin{tabular}{lccc}
            \toprule[2pt]
            \multirow{2}{*}{\bf{Dataset}} &
            \multicolumn{3}{c}{\bf{\# Proteins}}\\
            & \bf{\# Train} & \bf{\# Validation} & \bf{\# 30\% Test / \# 50\% Test / \# 95\% Test}\\
            \midrule[1pt]
            \bf{Enzyme Commission} & 15,550 & 1,729 & 720 / 1,117 / 1,919 \\
            \bf{Gene Ontology} & 29,898 & 3,322 & 1,717 / 2,199 / 3,416 \\
            \bf{Fold Classification} & 12,312 & - & - \\
            \bottomrule[2pt]
        \end{tabular}
    \end{adjustbox}
\end{table}

Dataset statistics are summarized in Table~\ref{tab:dataset}.
Details are introduced as follows.

For evaluation, we adopt two standard function annotation tasks as in previous works~\citep{gligorijevic2021structure,zhang2022protein}.
The first task, Enzyme Commission (EC) number prediction, involves forecasting the EC numbers for proteins, categorizing their role in catalyzing biochemical reactions.
We have focused on the third and fourth levels of the EC hierarchy~\citep{webb1992enzyme}, forming 538 distinct binary classification challenges.
The second task, Gene Ontology (GO) term prediction, targets the identification of protein associations with specific GO terms. We select GO terms that have a training sample size between 50 and 5000.
These terms are part of a classification that organizes proteins into functionally related groups within three ontological categories: molecular function (MF), biological process (BP), and cellular component (CC).

To construct a non-redundant dataset, all PDB chains are clustered, setting a 95\% sequence identity threshold. From each cluster, a representative PDB chain is chosen based on two criteria: annotation presence (at least one GO term from any of the three ontologies) and high-quality structural resolution.
The non-redundant sets are divided into training, validation and test sets with approximate ratios 80/10/10\%.
The test set exclusively contains experimentally verified PDB structures and annotations.
We ensure that these PDB chains exhibit a varied sequence identity spectrum relative to the training set, specifically at 30\%, 50\%, and 95\% sequence identity levels. Moreover, each PDB chain in the test set is guaranteed to have at least one experimentally validated GO term from each GO category.

For pre-training a protein structure retriever, we adopt the fold classfication task~\citep{hou2018deepsf}, which holds significant relevance in analyzing the relationship between protein structure and function, as well as in the exploration of protein evolution~\citep{hou2018deepsf}. This classification groups proteins based on the similarity of their secondary structures, their spatial orientations, and the sequence of their connections. The task requires predicting the fold class to which a given protein belongs.

\begin{table*}[t]
    \centering
    \caption{F\textsubscript{max} on EC and GO prediction with predictors and retrievers based on PLMs.
    }
    \vspace{-0.8em}
    \label{tab:esm}
    \begin{threeparttable}
    \begin{adjustbox}{max width=\linewidth}
        \begin{tabular}{lcccccccccccccccccc}
            \toprule[2pt]
            & \multirow{2}{*}{\large{\bf{ Method}}} &&
            \multicolumn{3}{c}{\bf{EC}}&&
            \multicolumn{3}{c}{\bf{GO-BP}} && 
            \multicolumn{3}{c}{\bf{GO-MF}} && 
            \multicolumn{3}{c}{\bf{GO-CC}}
            \\
            \cmidrule{4-6}
            \cmidrule{8-10}
            \cmidrule{12-14}
            \cmidrule{16-18}
            & && 30\% & 50\% & 95\% &&
            30\% & 50\% & 95\% && 
            30\% & 50\% & 95\% && 
            30\% & 50\% & 95\% 
            \\
            \midrule[1.5pt]
            \multirow{4}{*}{\rotatebox{90}{\bf{Predictor}}}
            % & {ESM-1b} && \multicolumn{3}{c}{\textcolor{red}{TODO}} && \multicolumn{3}{c}{\textcolor{red}{TODO}} && \multicolumn{3}{c}{\textcolor{red}{TODO}} && \multicolumn{3}{c}{\textcolor{red}{TODO}}\\
            & {ESM-2-8M} && 0.510 & 0.565 & 0.658 && 0.323 & 0.331 & 0.368 && 0.395 & 0.427 & 0.502 && 0.417 & 0.431 & 0.457\\
            & {ESM-2-35M} && 0.678 & 0.744 & 0.818 && 0.382 & 0.393 & 0.443 && 0.493 & 0.533 & 0.610 && 0.444 & 0.457 & 0.481\\
            & {ESM-2-150M} && 0.749 & 0.802 & 0.865 && 0.397 & 0.413 & 0.460 && 0.558 & 0.599 & 0.667 && {0.481} & 0.493 & {0.523}\\
            & {ESM-2-650M} && \textcolor{red}{\bf{0.763}} & \textcolor{red}{\bf{0.816}} & \textcolor{red}{\bf{0.877}} && \textcolor{blue}{\bf{0.423}} & \textcolor{blue}{\bf{0.438}} & \textcolor{blue}{\bf{0.484}} && \textcolor{blue}{\bf{0.563}} & \textcolor{blue}{\bf{0.604}} & \textcolor{blue}{\bf{0.661}} && \textcolor{red}{\bf{0.497}} & \textcolor{red}{\bf{0.509}} & \textcolor{red}{\bf{0.535}}\\
            \midrule[1.5pt]
            \multirow{8}{*}{\rotatebox{90}{\bf{Retriever}}}
            % & {ESM-1b} && 0.525 & 0.563 & 0.627 && 0.280 & 0.304 & 0.355 && 0.428 & 0.467 & 0.532 && 0.274 & 0.274 & 0.288\\
            & {ESM-2-8M} && 0.423 & 0.449 & 0.581 && 0.337 & 0.355 & 0.423 && 0.420 & 0.455 & 0.553 && 0.359 & 0.367 & 0.413\\
            & {ESM-2-35M} && 0.428 & 0.436 & 0.560 && 0.390 & 0.411 & 0.471 && \bf{0.485} & \bf{0.531} & \bf{0.618} && 0.402 & 0.410 & 0.448\\
            & {ESM-2-150M} && 0.482 & 0.538 & 0.656 && 0.383 & 0.404 & 0.468 && {0.467} & {0.516} & {0.611} && 0.415 & 0.427 & 0.462\\
            & {ESM-2-650M} && \bf{0.585} & \bf{0.656} & \bf{0.753} && \bf{0.398}& \bf{0.415} & \bf{0.477} && 0.462 & 0.510 &	0.607 && \bf{0.427} & \bf{0.436} & \bf{0.472}\\
            \cmidrule{2-18}
            & \bf{ESM-2-8M \emph{w/ struct.}} && 0.482 & 0.499 & 0.620 && 0.368 & 0.389 & 0.453 && 0.461 & 0.504 & 0.596 && 0.377 & 0.392 & 0.433\\
            & \bf{ESM-2-35M \emph{w/ struct.}} && 0.502 & 0.553 &  0.658 && 0.417 & 0.439 & 0.494 && 0.522 & 0.570 & 0.649 && 0.414 & 0.425 & 0.459\\
            & \bf{ESM-2-150M \emph{w/ struct.}} && 0.547 & 0.598 & 0.690 && 0.434 & 0.455 & 0.506 && 0.548 & 0.594 & 0.666 && 0.424 & 0.436 & 0.472\\
            & \bf{ESM-2-650M \emph{w/ struct.}} && \textcolor{blue}{\bf{0.676}} & \textcolor{blue}{\bf{0.742}} &  \textcolor{blue}{\bf{0.817}} && \textcolor{red}{\bf{0.455}} & \textcolor{red}{\bf{0.472}} & \textcolor{red}{\bf{0.519}} && \textcolor{red}{\bf{0.570}} & \textcolor{red}{\bf{0.612}} &	\textcolor{red}{\bf{0.678}} && \textcolor{blue}{\bf{0.448}} & \textcolor{blue}{\bf{0.455}} & \textcolor{blue}{\bf{0.485}}\\
            \midrule[1.5pt]
            \multicolumn{2}{c}{PromptProtein}  && {0.765} & {0.823} & {0.888} && {0.439} & {0.453} & {0.495} && {0.577} & {0.600} & {0.677} && {0.532} & {0.533} & {0.551} \\
            \midrule
             \multicolumn{2}{c}{\bf{ESM-2-650M ensemble}} && 0.768 & 0.819 & 0.879 && 0.459 & 0.472 & 0.516 && 0.588 & 0.627 & 0.690 && 0.506 & 0.514 & 0.540\\
            \bottomrule[2pt]
        \end{tabular}
    \end{adjustbox}
    \begin{tablenotes}
        \item[*] \footnotesize \textcolor{red}{\bf{Red}}: the best results among all; \textcolor{blue}{\bf{blue}}: the second best results among all; \textbf{bold}: the best results within blocks.
    \end{tablenotes}
    \end{threeparttable}
\end{table*}
